# Supplementary material for: Interpersonal trust: Asymptotic analysis of a stochastic coordination game with multi-agent learning
Source: arXiv:2402.03894 source file (2024-05-17)
Supplement: Supplementary file 1 [file appendix.tex]

%%%% 
% In this tex file I include as appendices the sketches for how to prove our results on general (complex) networks. This may be useful for submitting it to `the Journal of Complex Networks' which I think is a good place for it once Chaos rejects it.
%%%%

\section{Sketch of procedure to prove Lemma~\ref{lem:stay0N} and Lemma~\ref{lem:stay1N} for general connected networks}\label{sec:stay_gen}
The event described by this lemma (absorption at zero and one) requires all agents to take the same action indefinitely: defect for absorption at $\bm{0}^n$ and cooperate for absorption at $\bm{1}^n$. For the purposes of illustrating the procedure we consider only absorption at $\bm{0}^n$.

The proof is by induction on the number of agents in the connected network with $n=2$ as the base case which may be proved in exactly the same way as is done in the proof of Lemma~\ref{lem:stay0N}.
%One sets up an infinite product where each term represents the probability that both agents take the defect action per round of matches. This infinite product can be shown to converge by transforming it into an infinite sum (taking logarithms) and applying Abel's convergence test (cf. \cite{Whittaker1920}). 

For the induction step we take a vertex cover $\mathcal{V}$ of the network. We set up another infinite product in which each term corresponds to the probability that the chosen agents play the defect action in each match. Because there are an infinite number of games, we know that each of the vertex will play each of their neighbours an infinite number of times. In particular each agent in $\mathcal{V}$ will play each of their neighbours an infinite number of times. We can split up the product with the games ordered chronologically into a product in which the games are ordered according to matches between general agents and agents in $\mathcal{V}$. By arguments similar to how the base case was proved to converge, this product of products can be shown to converge.

\section{Sketch of procedure to prove Lemma~\ref{lem:n_reach0} and Lemma~\ref{lem:n_reach1} for general connected networks}\label{sec:reach_gen}
To prove that there is positive probability of reaching the $\epsilon$-balls around $\bm{0}^n$ and $\bm{1}^n$ respectively one delineates a sequence of events which lead to this outcome.
%We discuss the changes to the proof of Lemma~3 in~\cite{Meylahn2024} which focuses
We focus on reaching the $\epsilon$-ball at $\bm{0}^n$.

This may be proved by choosing a match-up between pairs of agents in the population. In the fully connected network one has a lot of freedom, but in the general connected networks we have to be a little more careful. If there exists an perfect matching (a set of edges such that each agent is connected to exactly one edge in the covering) then the proof may proceed exactly like the proof of Lemma~\ref{lem:n_reach0}. Therein each pair of agents are chosen to play against one another a finite number of times with positive probability and take the defect action each time with positive probability.

%To clarify the number of matches they each should play in their pairing is:
%\begin{equation}\label{eq:k_finite}
 %   \kappa = \bigg\lceil \frac{\log (\epsilon/x_i(t_0))}{\log  (1-\alpha)}\bigg\rceil,
%\end{equation}
%after playing $\kappa$ matches and observing (and playing) defect each time, both agents in the matchup have belief $x<\epsilon$.

If there is no perfect matching we take instead, an edge cover $\mathcal{E}$. We take a matching (not perfect) from this edge cover and for these agents we may follow the same procedure as before. The agents that were not a part of this matching, are then considered separately. We pair them up to play a game against their neighbour in $\mathcal{E}$ $\kappa$ times. They play defect with positive probability and of course because their neighbours have already gone through this procedure once, they too play defect each time with positive probability. 

Edge cases in which only one agent has belief $x<1-\epsilon$ and all other $x=1$ may be handled by constructing a spanning tree rooted at the agent who has belief $x<1-\epsilon$. Then in increasing order of depth, each agent plays three games against the parent in the tree. In the first only the parent plays defect, in the second, the child plays defect and in the third they both play defect with positive probability. Then they both have belief $x<1-\epsilon$.
